# Supplementary material for: Interplay between ferroelectricity and metallicity in hexagonal YMnO$_3$
Source: arXiv:2406.01537 source file (2024-06-03)
Supplement: Supplementary file 1 [file suppinfo.pdf]

# Supplementary Information

Tara N. Tošić,[*] Yuting Chen, and Nicola A. Spaldin[†]
*Materials Theory, ETH Zürich, Wolfgang-Pauli-Strasse 27, 8093 Zurich, Switzerland*

[*] tara.tosic@mat.ethz.ch
[†] nspaldin@ethz.ch

### A. Determining $U$ using the Linear Response Ansatz

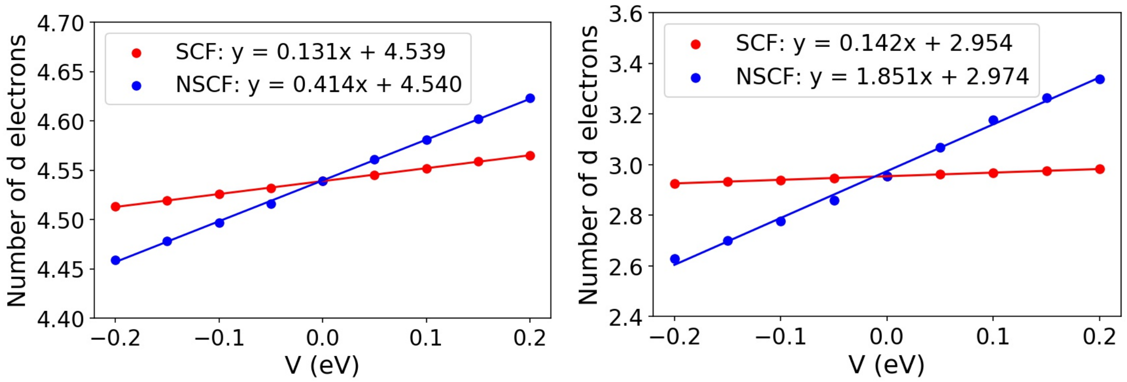


FIG. S1: Number of $d$ electrons at small value of on-site potential for Mn (left) and V (right) in h-$YMnO_3$ structure.

To obtain $U$ for a given element, we perform self-consistent (SCF) and non self-consistent (NSCF) calculations separately and apply a small on-site potential V to the target atom. The $U$ parameter is calculated as the difference between the reciprocal of density response functions ($\chi$) [33]:

$$U = \chi^{-1} - \chi_0^{-1} \approx \left(\frac{\partial N_I^{SCF}}{\partial V_I}\right)^{-1} - \left(\frac{\partial N_I^{NSCF}}{\partial V_I}\right)^{-1}. \tag{1}$$

In Figure S1, we plot the number of $d$ electrons versus the potential in the 30-atom unit cell. The $U$ parameters for Mn $d$ orbital and V $d$ orbital are 5.2 eV and 6.5 eV respectively. Given the improper nature of the ferroelectricity and its coupling to the primary $K_3$ mode which affects the $spd^3$ orbital hybridization of the $MnO_5$, we opt for this method to optimize $U$ [33]. It allows us to correct for the erroneous curvature of the total energy as a function of non-integer occupation of electronic orbitals, and thus describe the orbitals involved in the improper FE transition more accurately..

### B. Projected DOS at other background charge doping concentrations

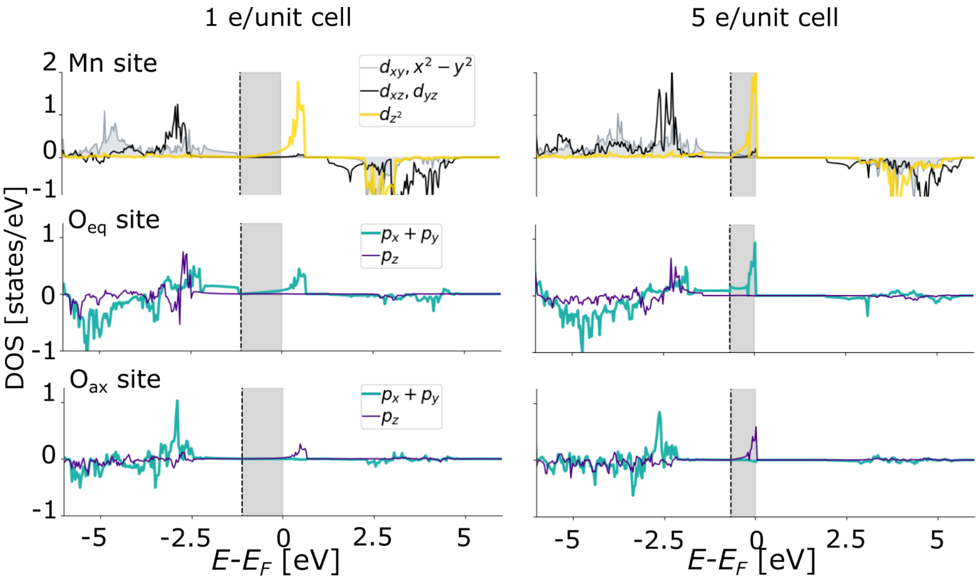


FIG. S2: Additional DOS plots for intermediate (1e/unit cell) and higher (5e/unit cell) values of electron doping.

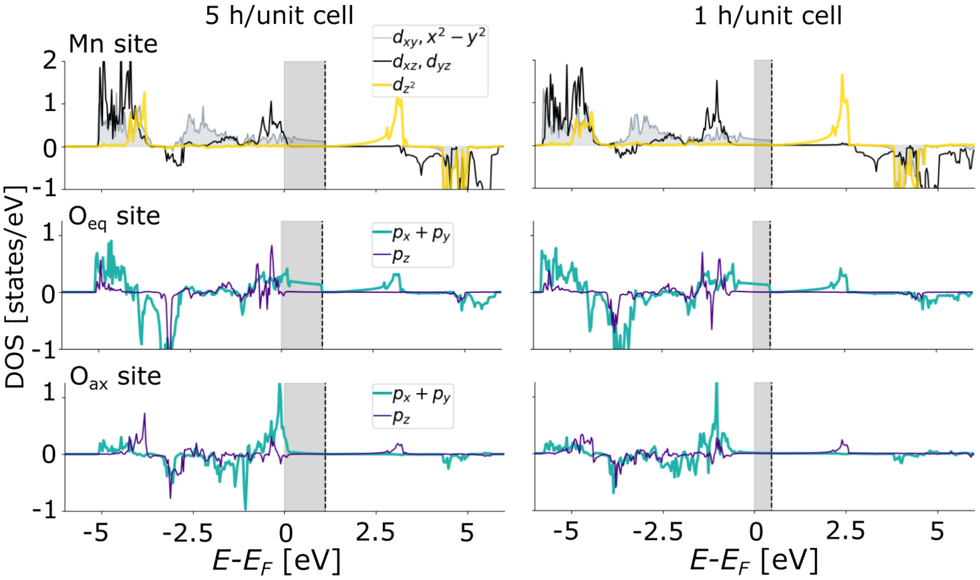


FIG. S3: Additional DOS plots for intermediate (1h/unit cell) and higher (5h/unit cell) values of hole doping.
